# Supplementary material for: Quantitative three-dimensional local order analysis of nanomaterials through electron diffraction
Source: arXiv:2305.02180 source file (2023-05-03)
Supplement: Supplementary file 1 [file Supplement.pdf]

# Quantitative three-dimensional local order analysis of nanomaterials through electron diffraction

## SUPPORTING INFORMATION

Ella M. Schmidt*, Paul B. Klar, Yaşar Krysiak, Petr Svora, Andrew L. Goodwin and Lukas Palatinus

*E-mail: ella.schmidt@uni-bremen.de

# Contents

**1 Ion milled sample for electron diffraction measurements** **S3**

**2 Reciprocal space coverage** **S3**

**3 Parameters for data treatment** **S5**

X-ray and neutron diffraction . . . . . . . . . . . . . . . . . . . . . . . . . . . . . . S5

Electron diffraction . . . . . . . . . . . . . . . . . . . . . . . . . . . . . . . . . . . . S5

**4 Two dimensional sections of the shortest vectors** **S6**

**5 Three dimensional fits** **S8**

$\left(\frac{1}{2},0,0\right)$ interatomic vector . . . . . . . . . . . . . . . . . . . . . . . . . . . . . S8

$\left(\frac{1}{4},\frac{1}{4},\frac{1}{4}\right)$ interatomic vector . . . . . . . . . . . . . . . . . . . . . . . . . . . . S9

$\left(\frac{1}{2},\frac{1}{2},0\right)$ interatomic vector . . . . . . . . . . . . . . . . . . . . . . . . . . . . S9

**6 Relative ratio of the form factors** **S11**

**7 Model** **S12**

**8 References** **S15**

## 1 Ion milled sample for electron diffraction measurements

Figure S1 shows the top view of the ion milled sample prepared for the electron diffraction experiments. The estimated thickness range of the sample is 40 to 60 nm. Residual Ga ions from ion milling could penitentially be in-cooperated on the sample surface.

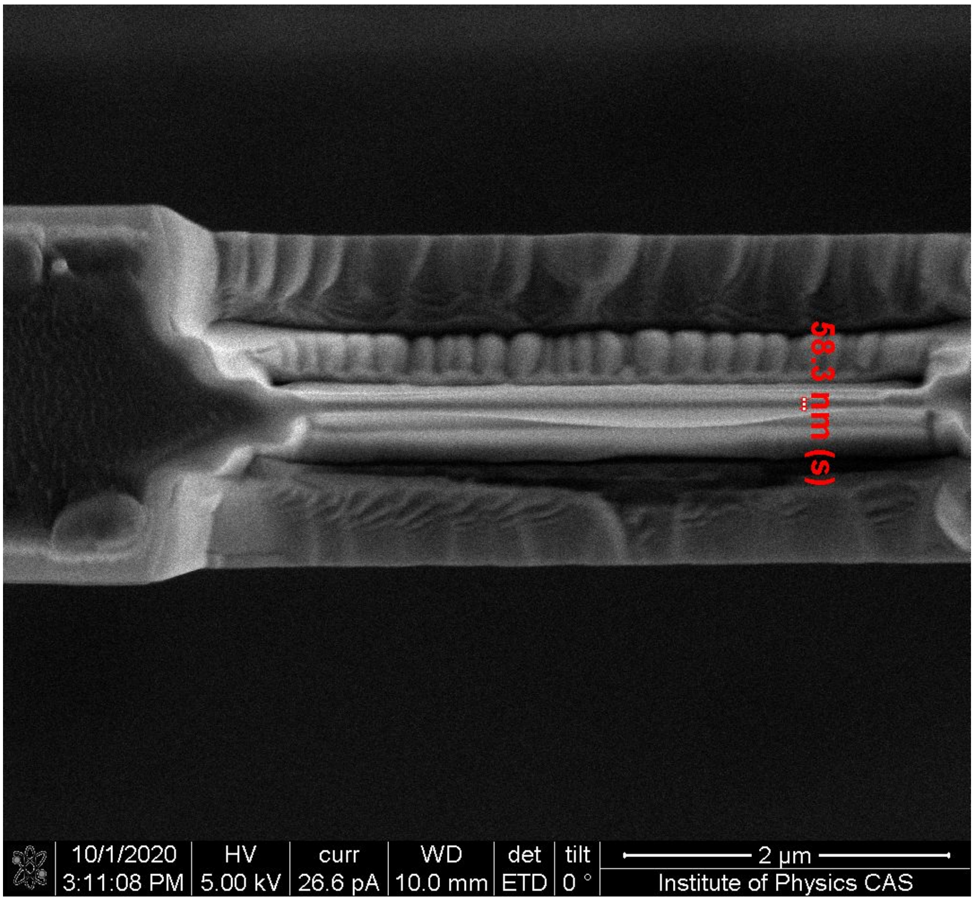


**Figure S1:** SEM image of the ion milled sample prepared for electron diffraction experiments.

## 2 Reciprocal space coverage

Figure S2 shows the reciprocal space coverage before and after symmetry averaging for the three performed diffraction experiments. In the electron diffraction experiment $\approx 28$ % of reciprocal space were measured. Due to the limited goniometer tilt range in the missing wedge in the data is clearly observed. The neutron diffraction experiment was conducted using a 180 deg $\phi$-scan, which yields a reciprocal space coverage of $\approx 50$ %. For x-ray diffraction several $\omega$-scans were conducted, which yield 100 % reciprocal space coverage in the considered resolution range. The high $m\bar{3}m$ Laue symmetry allows to fill any remaining gaps by symmetry equivalent data.

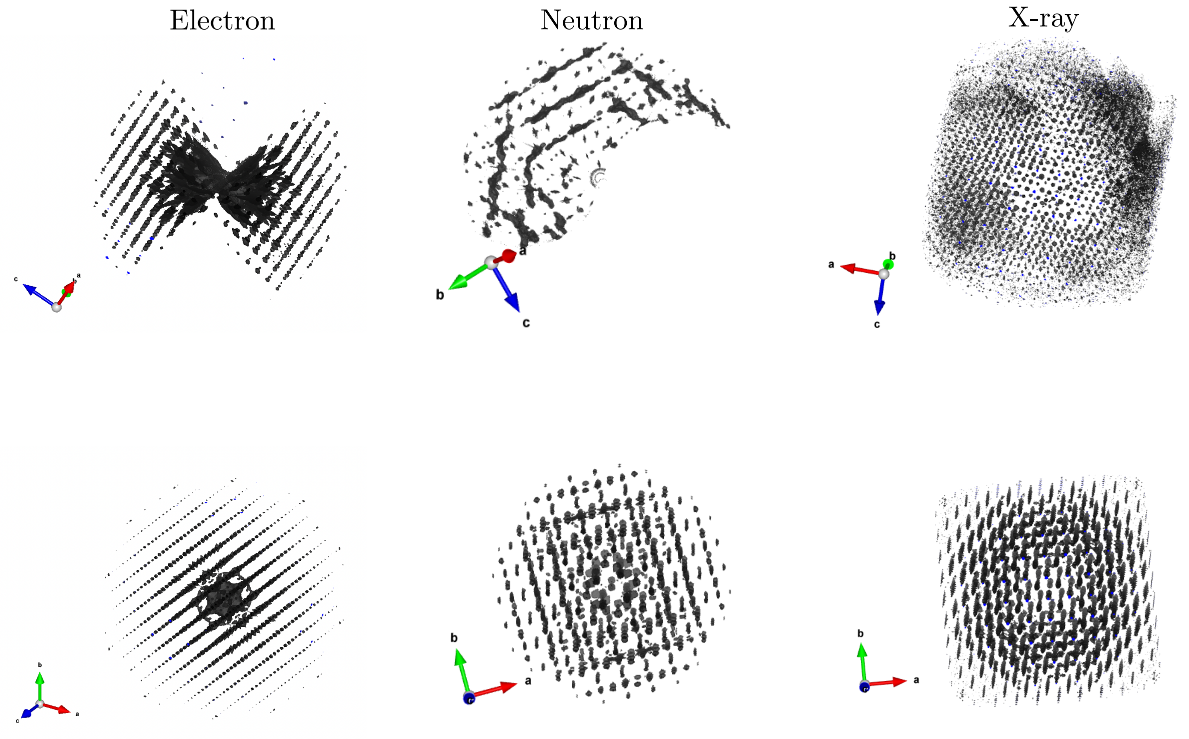


**Figure S2:** Three dimensional renderings of the reconstructed diffraction space for the electron, neutron and x-ray diffraction experiment. Top before and bottom after symmetry averaging for $m\bar{3}m$ Laue symmetry.

## 3 Parameters for data treatment

### X-ray and neutron diffraction

The data treatment for x-ray and neutron diffraction experiments was identical. Reciprocal space was reconstructed on a grid of $501 \times 501 \times 501$ voxels with $-10 \leq h, k, l \leq 10$. For the Karen[S1] algorithm a median window width of 5 voxels was chosen. The Bragg peaks that fulfil the F-centring diffraction conditions were punched with a sphere with a punch radius of 8 voxels. To interpolate the missing intensity the SciPy[S2] interpolation of grid-data was used with a mutiquadratic function (Rbf with parameters smooth=2.5, epsilon=2.5 ). For the Gaussian falloff to reduce finite size ripples in the Fourier transform for each voxel the distance $d$ in voxels to the centre of reciprocal space was calculated and its intensity multiplied with $\exp(-7.5 \cdot 10^{-5} \cdot d^2)$.

### Electron diffraction

Reciprocal space was reconstructed on a grid of $201 \times 201 \times 201$ voxels with $-10 \leq h, k, l \leq 10$. For the Karen[S1] algorithm a median window width of 5 voxels was chosen. The Bragg peaks that fulfil the F-centring diffraction conditions were punched with a sphere with a punch radius of 5 voxels. On an absolute scale this corresponds to a much larger sphere than in the case for x-ray and neutron diffraction. To interpolate the missing intensity the SciPy[S2] interpolation of grid-data was used with a mutiquadratic function (Rbf with parameters smooth=2.5, epsilon=2.5 ). For the Gaussian falloff to reduce finite size ripples in the Fourier transform for each voxel the distance $d$ in voxels to the centre of reciprocal space was calculated and its intensity multiplied with $\exp(-1.25 \cdot 10^{-4} \cdot d^2)$. This is the same relative dampening as applied to the x-ray and neutron data.

The electron diffraction experiment did not use a beam stop. Therefore the central region of reciprocal space also includes a halo of the primary electron beam on the detector. To subtract the contributions of the primary beam the punched and filled data was radially integrated and approximated with a sum of two Gaussian functions. The FWHM of these Gaussians is much wider than for typical diffuse scattering features. This background was subsequently subtracted from the diffraction data before Fourier transforming.

# 4 Two dimensional sections of the shortest vectors

Two dimensional sections of the shortest interatomic vectors are shown in Figures S3, S4, S5 and S6.

**Figure S3:** 3D-ΔPDFs obtained from x-ray (left), neutron (middle) and electron (right) diffraction experiments. Two-dimensional plot in the $ab0$-layer. Dotted lines indicate the average interatomic vector at $\left(\frac{1}{2},0,0\right)$. Positive intensities in red, negative intensities in blue.

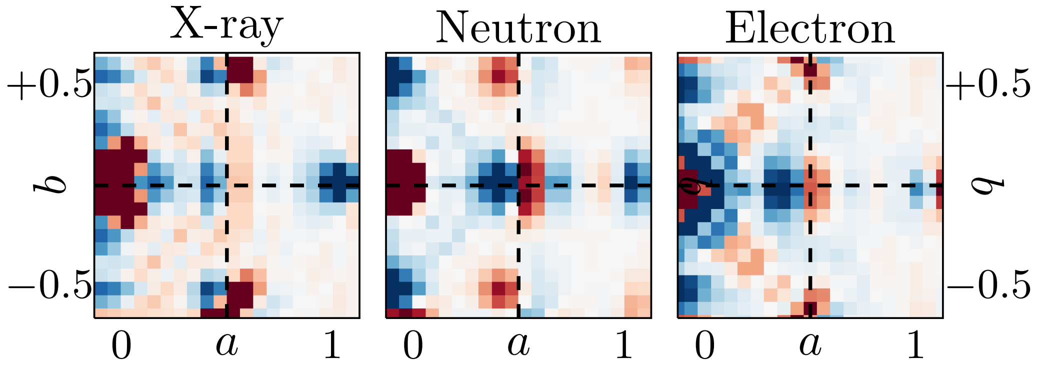


**Figure S4:** 3D-ΔPDFs obtained from x-ray (left), neutron (middle) and electron (right) diffraction experiments. Two-dimensional plot in the $ab0.25$-layer. Dotted lines indicate the average interatomic vector at $\left(\frac{1}{4},\frac{1}{4},\frac{1}{4}\right)$. Positive intensities in red, negative intensities in blue.

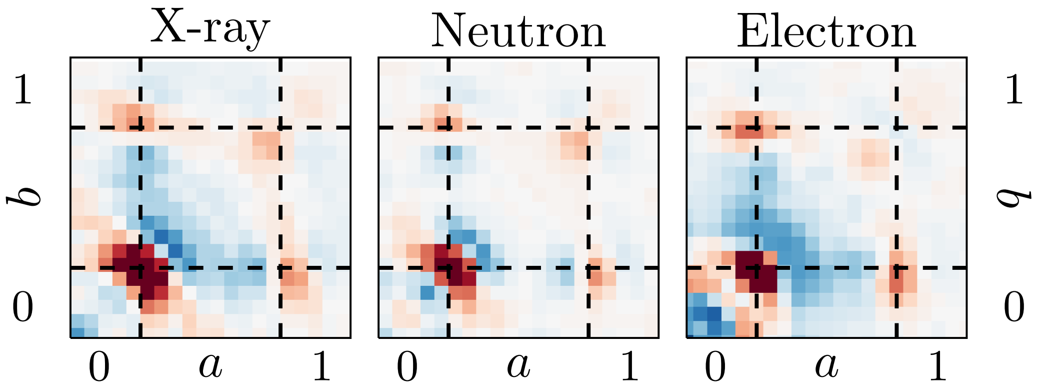

**Figure S5:** 3D-ΔPDFs obtained from x-ray (left), neutron (middle) and electron (right) diffraction experiments. Two-dimensional plot in the $ab0$-layer. Dotted lines indicate the average interatomic vector at $\left(\frac{1}{2},\frac{1}{2},0\right)$. Positive intensities in red, negative intensities in blue.

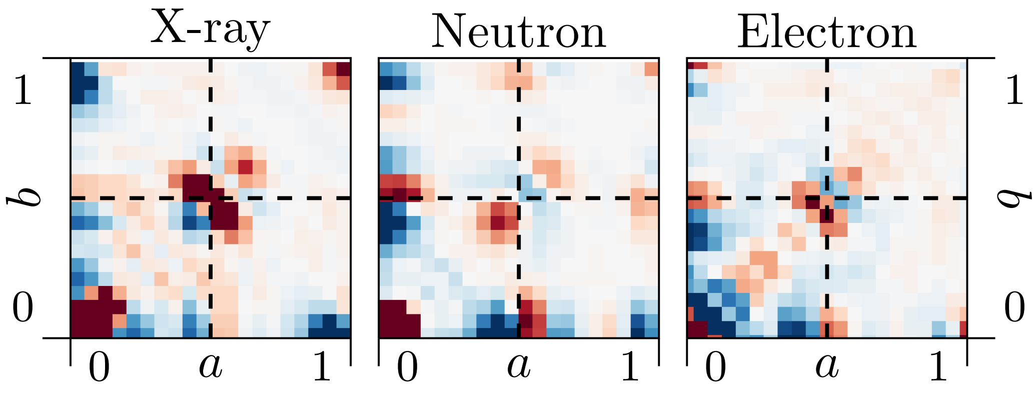


**Figure S6:** 3D-ΔPDFs obtained from x-ray (left), neutron (middle) and electron (right) diffraction experiments. Two-dimensional plot in the $ab0.5$-layer. Dotted lines indicate the average interatomic vector at $\left(\frac{1}{2},\frac{1}{2},\frac{1}{2}\right)$. Positive intensities in red, negative intensities in blue.

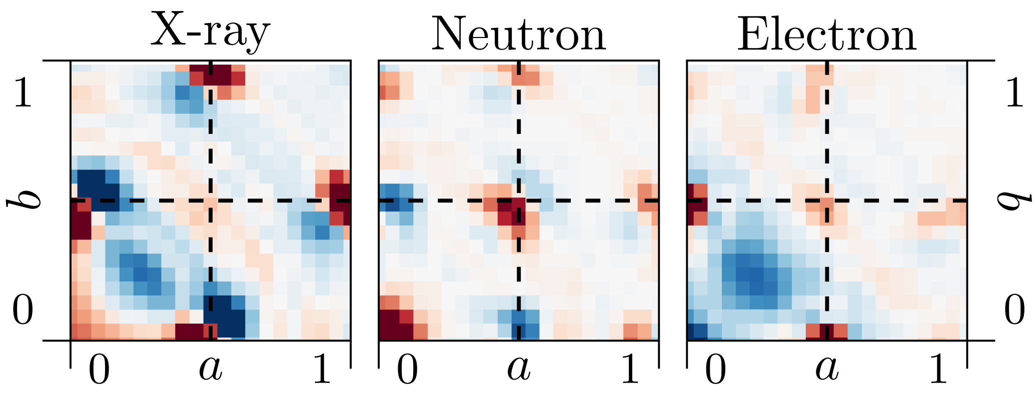

## 5 Three dimensional fits

The position of several maxima and minima in the 3D-Δ PDFs were refined by approximating the intensity distribution as three-dimensional Gaussian distributions. For this purpose the Voronoi cell around each of the shortest interatomic vectors was extracted from the data. Positive and negative intensities were treated separately. For all interatomic vectors a function of the form

$$I(\vec{x}) = I_0 \cdot \exp\left(-\frac{1}{2}(\vec{x}-\vec{x}_0)^T \underline{\underline{M}}(\vec{x}-\vec{x}_0)\right) \tag{1}$$

was fitted to the intensity distribution.

### $\left(\frac{1}{2},0,0\right)$ interatomic vector

As the observed intensity distribution around the $\left(\frac{1}{2},0,0\right)$ interatomic vector is rotationally symmetric around the $a$-axis the number of free parameters in Equation 1 was reduced to four: $\vec{x}_0$ was restricted to $\left(\frac{1}{2}+\Delta,0,0\right)$ and $\underline{\underline{M}}$ was restricted to

$$\underline{\underline{M}} = \begin{pmatrix} m_{11} & 0 & 0 \\ 0 & m_{22} & 0 \\ 0 & 0 & m_{22} \end{pmatrix}.$$

The resulting parameters are listed in Table S1.

**Table S1:** Refined parameters for the Gaussian distribution the observed maxima and minima away from the average $\left(\frac{1}{2},0,0\right)$ interatomic vector.

| | $I_0$ [arb. u.] | $\Delta^+$ [r.l.u.] | $m_{11}$ [(r.l.u)$^{-2}$] | $m_{22}$ [(r.l.u)$^{-2}$] |
|---|---|---|---|---|
| | | Maximum | | |
| $e^-$ | 3.10(109) | $2.19(16) \cdot 10^{-2}$ | $2.29(114) \cdot 10^{3}$ | $1.66(4) \cdot 10^{2}$ |
| $\gamma$ | 0.481(3) | $2.28(17) \cdot 10^{-2}$ | $0.71(8) \cdot 10^{3}$ | $0.63(7) \cdot 10^{2}$ |
| $n$ | 5.36(13) | $1.71(5) \cdot 10^{-2}$ | $1.09(5) \cdot 10^{3}$ | $1.03(3) \cdot 10^{2}$ |
| | | Minimum | | |
| $e^-$ | -3.36(5) | $-1.17(1) \cdot 10^{-1}$ | $3.19(19) \cdot 10^{2}$ | $1.39(4) \cdot 10^{2}$ |
| $\gamma$ | -1.31(3) | $-0.92(1) \cdot 10^{-1}$ | $12.05(53) \cdot 10^{2}$ | $1.38(4) \cdot 10^{2}$ |
| $n$ | -7.83(25) | $-1.02(1) \cdot 10^{-1}$ | $6.22(3) \cdot 10^{2}$ | $3.11(13) \cdot 10^{2}$ |

## $\left(\frac{1}{4}, \frac{1}{4}, \frac{1}{4}\right)$ interatomic vector

For the purpose of the fit the intensity distribution was approximated as rotationally symmetric around the [111]-direction. The number of free parameters was reduced to four: $\vec{x}_0$ was restricted to $\left(\frac{1}{4}+\Delta, \frac{1}{4}+\Delta, \frac{1}{4}+\Delta\right)$ and $\underline{\underline{M}}$ was restricted to

$$\underline{\underline{M}} = \begin{pmatrix} m_{11} & m_{12} & m_{12} \\ m_{12} & m_{11} & m_{12} \\ m_{12} & m_{12} & m_{11} \end{pmatrix}.$$

The resulting parameters are listed in Table S2.

**Table S2:** Refined parameters for the Gaussian distribution the observed maxima and minima away from the average $\left(\frac{1}{4}, \frac{1}{4}, \frac{1}{4}\right)$ interatomic vector.

| | $I_0$ [arb. u.] | $\Delta^+$ [r.l.u.] | $m_{11}$ [(r.l.u)$^{-2}$] | $m_{12}$ [(r.l.u)$^{-2}$] |
|---|---|---|---|---|
| | | Maximum | | |
| $e^-$ | 10.27(28) | $-1.29(5) \cdot 10^{-2}$ | $4.95(17) \cdot 10^2$ | $2.35(16) \cdot 10^2$ |
| $\gamma$ | 28(8) | $-1.59(6) \cdot 10^{-2}$ | $3.18(12) \cdot 10^2$ | $1.54(11) \cdot 10^2$ |
| $n$ | 7.31(24) | $-9.97(52) \cdot 10^{-2}$ | $5.13(22) \cdot 10^2$ | $2.72(21) \cdot 10^2$ |
| | | Minimum | | |
| $e^-$ | -2.71(13) | $5.93(12) \cdot 10^{-2}$ | $1.85(13) \cdot 10^2$ | $1.13(12) \cdot 10^2$ |
| $\gamma$ | -1.44(6) | $6.45(9) \cdot 10^{-2}$ | $2.45(13) \cdot 10^2$ | $1.32(12) \cdot 10^2$ |
| $n$ | -2.88(28) | $4.98(14) \cdot 10^{-2}$ | $4.76(66) \cdot 10^2$ | $3.36(65) \cdot 10^2$ |

## $\left(\frac{1}{2}, \frac{1}{2}, 0\right)$ interatomic vector

In the neutron diffraction experiment the signatures of O-O correlations and those of metal-metal correlations are observable on similar absolute scales as the scattering lengths of oxygen and the metals are comparable. For x-ray and electron diffraction the metals dominate the 3D-ΔPDF map. We interpret the clear maximum at $\left(\frac{1}{2}+\Delta, \frac{1}{2}+\Delta, 0\right)$ as the signature of two metal ions that are both relaxed away along their respective $\langle 111 \rangle$ directions from a bridging vacancy. We refine the position of this maximum using a Gaussian distribution as described in Equation 1. To avoid the influence of the second larger maximum on the fit, the data in the

extracted voronoi cell is constrained to $a, b \geq 0.5$. In the neutron diffraction experiment, the signature shows a different shape, which is a clear indication that the oxygen ions also contribute in this case, hence a resulting fit position would not be comparable.

The number of free parameters was reduced to five: $\vec{x}_0$ was restricted to $\left(\frac{1}{2} + \Delta, \frac{1}{2} + \Delta, 0\right)$ and $\underline{\underline{M}}$ was restricted to

$$\underline{\underline{M}} = \begin{pmatrix} m_{11} & m_{12} & 0 \\ m_{12} & m_{11} & 0 \\ 0 & 0 & m_{33} \end{pmatrix}.$$

The resulting parameters are listed in Table S3.

**Table S3:** Refined parameters for the Gaussian distribution the observed maxima away from the average $\left(\frac{1}{2}, \frac{1}{2}, 0\right)$ interatomic vector.

| | $I_0$ [arb. u.] | $\Delta^+$ [r.l.u.] | $m_{11}$ [(r.l.u)$^{-2}$] | $m_{33}$ [(r.l.u)$^{-2}$] | $m_{12}$ [(r.l.u)$^{-2}$] ] |
|---|---|---|---|---|---|
| $e^-$ | 2.52(5) | $8.74(4) \cdot 10^{-2}$ | $7.55(20) \cdot 10^2$ | $6.69(20) \cdot 10^2$ | $2.74(20) \cdot 10^2$ |
| $\gamma$ | 1.24(3) | $10.43(4) \cdot 10^{-2}$ | $6.87(20) \cdot 10^2$ | $7.03(24) \cdot 10^2$ | $2.77(21) \cdot 10^2$ |

## 6 Relative ratio of the form factors

In Figure S7 the relative scattering power of O vs. Zr is visualised for the three different radiation types in the resolution range used in the experiments. Higher f(0)/f(Zr) or b(0)/b(Zr) indicates a contrast that is more favourable to detect lighter elements.

**Figure S7:** Ratio of atomic form factors and neutron scattering lengths for O vs. Zr for the three radiation types used in the experiment.

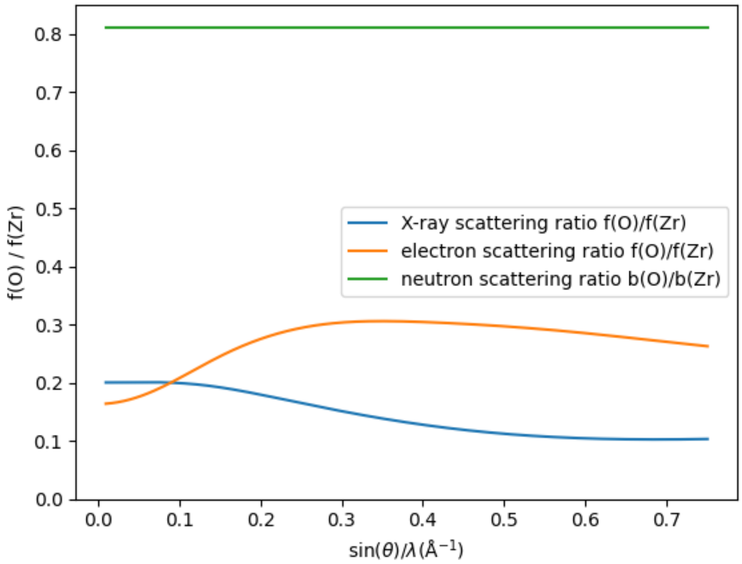

## 7 Model

We use the model that we established in our previous work[S3] to show that this also fits the electron diffraction results. We used Discus[S4] to calculate the scattering in the kinematic approximation. The resulting reciprocal $hk0$-layer, $hhl$-layer and real space $ab0$- and $aac$-sections are shown in Figures S8 and S9. Two-dimensional sections of the calculated and experimentally obtained 3D-ΔPDF around the shortest interatomic vectors are compared in S10. S11 compares the three-dimensional renderings of the model calculated for all three radiation types to the respective data.

**Figure S8:** Observed diffuse scattering compared to the calculated diffraction pattern of the model for electron diffraction in the kinematic approximation. (left) $hk0$-layer,(right) $hhl$-layer.

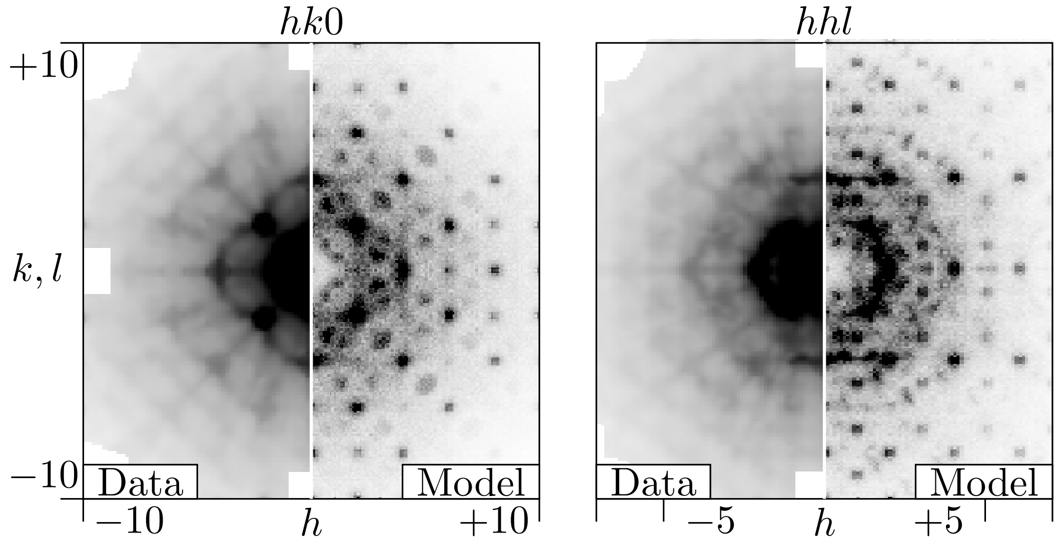

**Figure S9:** 3D-ΔPDF maps from the electron diffraction experiment compared to the model in kinematic approximations. (left) $ab0$-layer,(right) $aac$-layer.

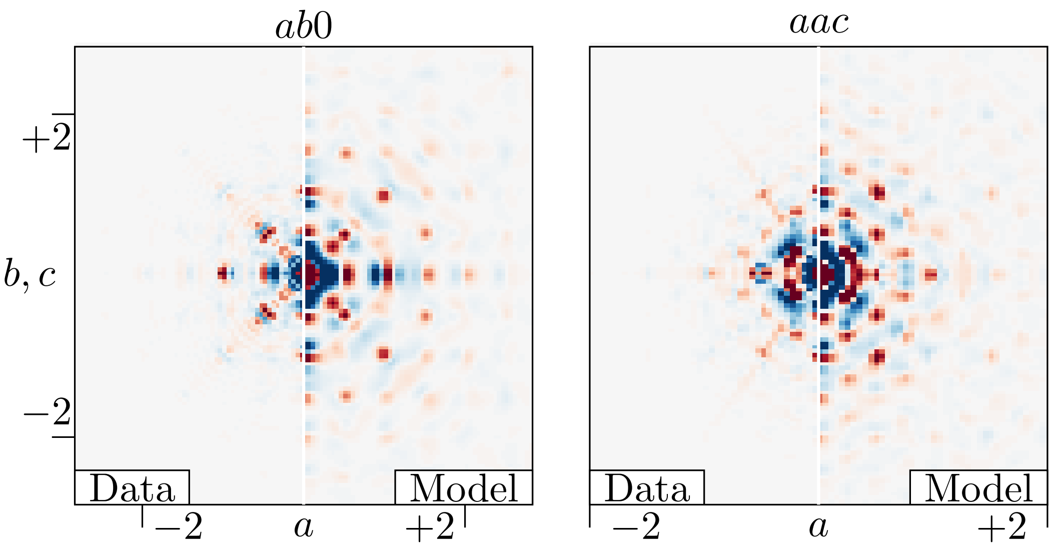


**Figure S10:** 3D-ΔPDFs obtained from a simplified model (M) compared to the experimentally obtained 3D-ΔPDFs (E). Three dimensional renderings are compared in Figure 4 of the main text. (a) Section around $\left(\frac{1}{2}, 0, 0\right)$ in the $ab0$-layer, model top, experiment bottom. (b) Section around $\left(\frac{1}{4}, \frac{1}{4}, \frac{1}{4},\right)$ in the $ab\frac{1}{4}$-layer, model top left, experiment bottom right. (c) Two-dimensional section around $\left(\frac{1}{2}, \frac{1}{2}, 0\right)$ in the $ab0$-layer model top left, experiment bottom right. (d) Two-dimensional section around $\left(\frac{1}{2}, \frac{1}{2}, \frac{1}{2}\right)$ in the $ab\frac{1}{2}$-layer, model top left, experiment bottom right

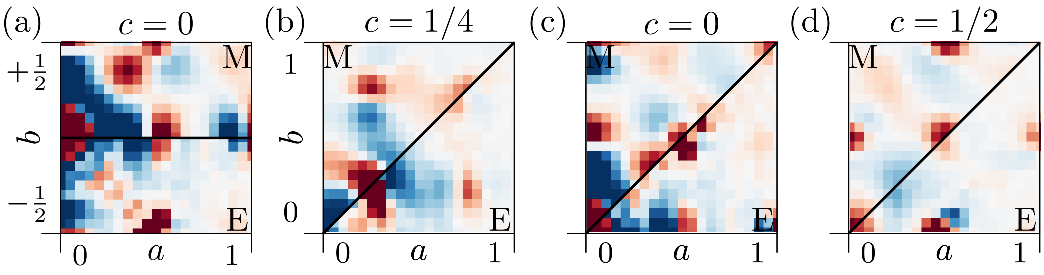

**Figure S11:** Three-dimensional renderings of the 3D-ΔPDFs calculated from the simplified model described in[S3] compared to the experimental data for all three radiation types used.

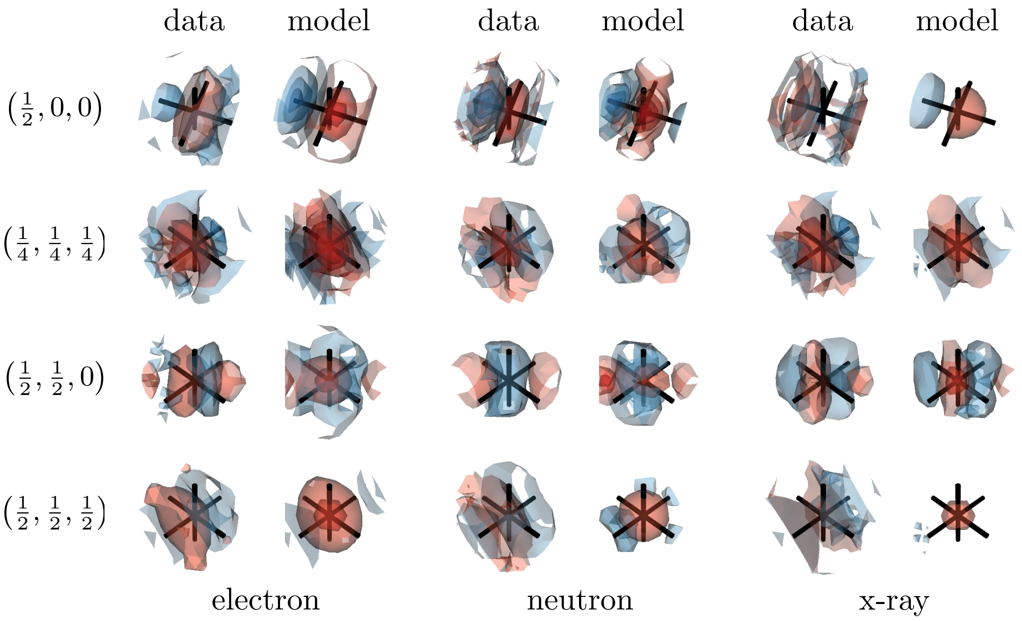

## 8 References


(S1) Weng, J. *et al.* K-space algorithmic reconstruction (karen): a robust statistical methodology to separate Bragg and diffuse scattering. *Journal of Applied Crystallography* **53** (1), 159–169 (2020).

(S2) Virtanen, Pauli, *et al.* SciPy 1.0: fundamental algorithms for scientific computing in Python. *Nature methods* **17**(3)3, 261-272 (2020).

(S3) Schmidt, E. M. *et al.* three-dimensional difference pair distribution functions (3D-ΔPDFs) of yttria-stabilized zirconia. *Acta Crystallographic Section B.* **79**(2), 138-147 (2023) .

(S4) Neder, R. B. & Proffen, T. *Diffuse Scattering and Defect Structure Simulations*, vol. 11. Oxford University Press. (2008).
